# Supplementary material for: Classifying bacteria clones using attention-based deep multiple instance learning interpreted by persistence homology
Source: arXiv:2012.01189 source file (2021-07-23)
Supplement: Supplementary file 1 [file bacteria_clones_wacv_supplement.tex]

\thispagestyle{empty}

%%%%%%%%%
In these supplementary materials, we first present additional sample images from the DIBaC database (see Fig.~\ref{fig:clone_examples}). We also present the average persistence bag of words for configurations $A$-$D$ and $B$-$D$ (see Fig.~\ref{fig:persist}). Moreover, we present standard and qualitative train confusion matrices obtained from representation and classification networks (see Fig.~\ref{fig:cm} and~\ref{fig:top_patches}). For the latter network, we additionally deliver receiver operating characteristics (see Fig.~\ref{fig:rocs}). Finally, we present the statistics on the number of bacteria and the number of connected components in AbMIL crucial patches (see Fig.~\ref{fig:bacteria_statistics}).
% \clearpage
\begin{figure}[ht]
\centering
\includegraphics[width=\linewidth]{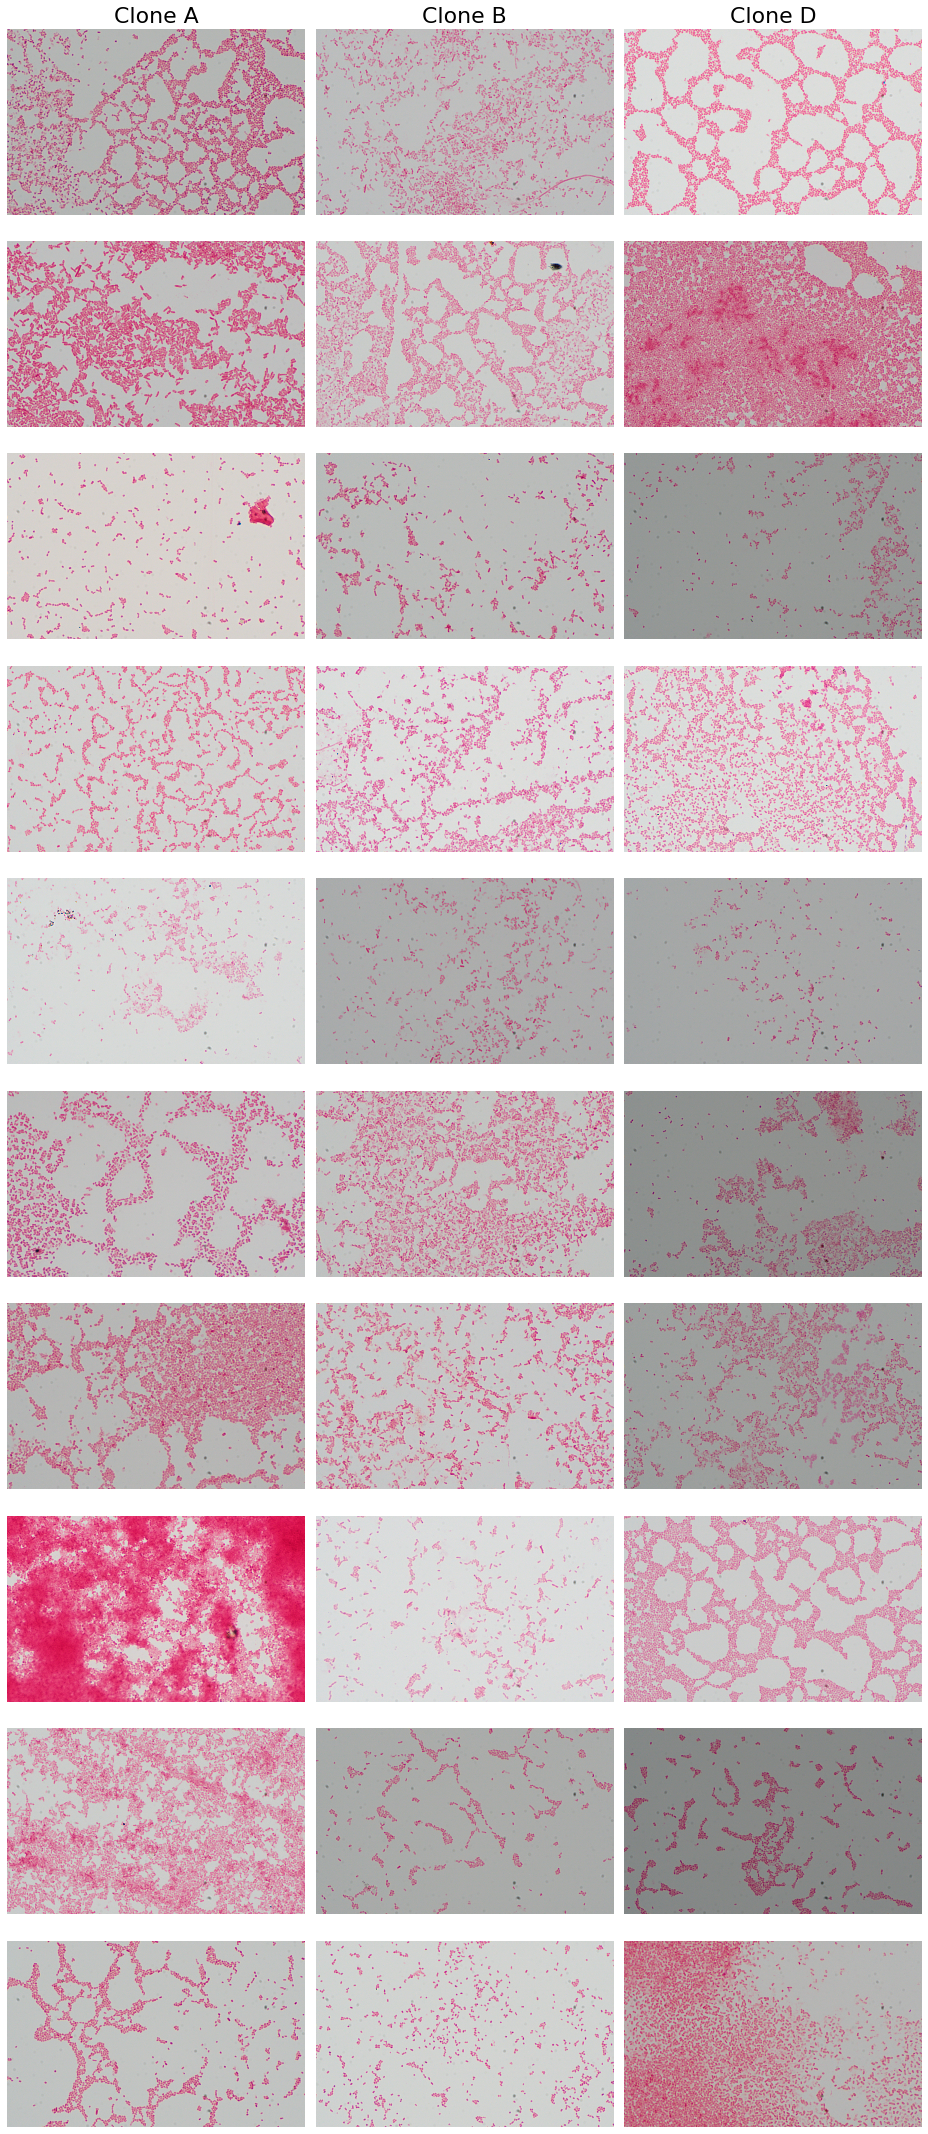}
\caption{Sample images from the DIBaC database ($10$ per clone).}
\label{fig:clone_examples}
\end{figure}

\begin{figure}[ht]
\centering
\begin{subfigure}[b]{0.9\linewidth}
  \centering
  \includegraphics[width=0.45\linewidth]{figures/AD_persistence_0_full.png}
  \includegraphics[width=0.45\linewidth]{figures/AD_persistence_0_full_pvalue.png}
  \caption{configuration $A$-$D$}
\end{subfigure}
\begin{subfigure}[b]{0.9\linewidth}
  \centering
  \includegraphics[width=0.45\linewidth]{figures/BD_persistence_0_full.png}
  \includegraphics[width=0.45\linewidth]{figures/BD_persistence_0_full_pvalue.png}
  \caption{configuration $B$-$D$}
\end{subfigure}
\caption{The average persistence bag of words for configurations $A$-$D$ and $B$-$D$ together with $0.99$ confidence interval (first column). The significance of difference is presented in the right column with a p-value of $0.01$ marked as the orange line.}
\label{fig:persist}
\end{figure}

\begin{figure}[ht]
\centering
\begin{subfigure}[b]{0.3\linewidth}
  \centering
  \includegraphics[width=\linewidth]{figures/cnn_cm_train_AB.png}
  \caption{repr. for $A$-$B$}
\end{subfigure}
\begin{subfigure}[b]{0.3\linewidth}
  \centering
  \includegraphics[width=\linewidth]{figures/cnn_cm_train_AD.png}
  \caption{repr. for $A$-$D$}
\end{subfigure}
\begin{subfigure}[b]{0.3\linewidth}
  \centering
  \includegraphics[width=\linewidth]{figures/cnn_cm_train_BD.png}
  \caption{repr. for $B$-$D$}
\end{subfigure}
\begin{subfigure}[b]{0.3\linewidth}
  \centering
  \includegraphics[width=\linewidth]{figures/abmilp_cm_avg_train_AB.png}
  \caption{class. for $A$-$B$}
\end{subfigure}
\begin{subfigure}[b]{0.3\linewidth}
  \centering
  \includegraphics[width=\linewidth]{figures/abmilp_cm_avg_train_AD.png}
  \caption{class. for $A$-$D$}
\end{subfigure}
\begin{subfigure}[b]{0.3\linewidth}
  \centering
  \includegraphics[width=\linewidth]{figures/abmilp_cm_avg_train_BD.png}
  \caption{class. for $B$-$D$}
\end{subfigure}
\caption{Train confusion matrices for representation and classification networks (first and second row, respectively) averaged over $5$ folds. Successive columns correspond to classifiers $A$-$B$, $A$-$D$, and $B$-$D$.}
\label{fig:cm}
\end{figure}

\begin{figure}[h]
\centering
\begin{subfigure}[b]{0.8\linewidth}
  \centering
  \includegraphics[width=\linewidth]{figures/abmilp_AB_valid.png}
  \caption{classifier $A$-$B$}
\end{subfigure}
\begin{subfigure}[b]{0.8\linewidth}
  \centering
  \includegraphics[width=\linewidth]{figures/abmilp_AD_valid.png}
  \caption{classifier $A$-$D$}
\end{subfigure}
\begin{subfigure}[b]{0.8\linewidth}
  \centering
  \includegraphics[width=\linewidth]{figures/abmilp_BD_valid.png}
  \caption{classifier $B$-$D$}
\end{subfigure}
\caption{Receiver operating characteristics (ROC) curves for each fold of AbMIL models.}
\label{fig:rocs}
\end{figure}

\begin{figure*}[ht]
\centering
\begin{subfigure}[b]{0.3\linewidth}
  \centering
  \includegraphics[width=\linewidth]{figures/cnn_patches_train_AB.png}
  \caption{representation net for $A$-$B$ case}
\end{subfigure}
\begin{subfigure}[b]{0.3\linewidth}
  \centering
  \includegraphics[width=\linewidth]{figures/cnn_patches_train_AD.png}
  \caption{representation net for $A$-$D$ case}
\end{subfigure}
\begin{subfigure}[b]{0.3\linewidth}
  \centering
  \includegraphics[width=\linewidth]{figures/cnn_patches_train_BD.png}
  \caption{representation net for $B$-$D$ case}
\end{subfigure}
\begin{subfigure}[b]{0.3\linewidth}
  \centering
  \includegraphics[width=\linewidth]{figures/patches_abmilp_AB_train.png}
  \caption{classifier net for $A$-$B$ case}
\end{subfigure}
\begin{subfigure}[b]{0.3\linewidth}
  \centering
  \includegraphics[width=\linewidth]{figures/patches_abmilp_AD_train.png}
  \caption{classifier net for $A$-$D$ case}
\end{subfigure}
\begin{subfigure}[b]{0.3\linewidth}
  \centering
  \includegraphics[width=\linewidth]{figures/patches_abmilp_BD_train.png}
  \caption{classifier net for $B$-$D$ case}
\end{subfigure}
\caption{Qualitative train confusion matrices obtained from representation and classification networks (first and second row, respectively) for fold $1$, where successive columns correspond to configurations $A$-$B$, $A$-$D$, and $B$-$D$. Each confusion matrix cell contains $9$ ($3 \times 3$) representative patches coming from different images.}
\label{fig:top_patches}
\end{figure*}

\begin{figure*}[ht]
\centering
\begin{subfigure}[b]{0.9\linewidth}
  \centering
  \includegraphics[width=0.3\linewidth]{figures/AB_hist_number_of_bacteria_full.png}
  \includegraphics[width=0.3\linewidth]{figures/AD_hist_number_of_bacteria_full.png}
  \includegraphics[width=0.3\linewidth]{figures/BD_hist_number_of_bacteria_full.png}
  \caption{number of bacteria per patch}
\end{subfigure}
\begin{subfigure}[b]{0.9\linewidth}
  \centering
  \includegraphics[width=0.3\linewidth]{figures/AB_hist_number_of_bacteria.png}
  \includegraphics[width=0.3\linewidth]{figures/AD_hist_number_of_bacteria.png}
  \includegraphics[width=0.3\linewidth]{figures/BD_hist_number_of_bacteria.png}
  \caption{number of bacteria per patch (same number of patches per bin for each clone)}
\end{subfigure}
\begin{subfigure}[b]{0.9\linewidth}
  \centering
  \includegraphics[width=0.3\linewidth]{figures/AB_hist_number_of_cc.png}
  \includegraphics[width=0.3\linewidth]{figures/AD_hist_number_of_cc.png}
  \includegraphics[width=0.3\linewidth]{figures/BD_hist_number_of_cc.png}
  \caption{number of connected components per patch limited to patches from (b)}
\end{subfigure}
\begin{subfigure}[b]{0.9\linewidth}
  \centering
  \includegraphics[width=0.3\linewidth]{figures/AB_hist_number_of_cc_by_bacteria.png}
  \includegraphics[width=0.3\linewidth]{figures/AD_hist_number_of_cc_by_bacteria.png}
  \includegraphics[width=0.3\linewidth]{figures/BD_hist_number_of_cc_by_bacteria.png}
  \caption{number of connected components / number of bacteria per patch limited to patches from (b)}
\end{subfigure}
\caption{Statistics on the number of bacteria and the number of connected components in AbMIL crucial patches. Successive columns correspond to classifiers $A$-$B$, $A$-$D$, and $B$-$D$.}
\label{fig:bacteria_statistics}
\end{figure*}

% \end{document}
